# Supplementary material for: FloVD: Optical Flow Meets Video Diffusion Model for Enhanced Camera-Controlled Video Synthesis
Source: arXiv:2502.08244 source file (2025-03-25)
Supplement: Supplementary file 1 [file X_suppl.tex]

\clearpage
\setcounter{page}{1}
\maketitlesupplementary

In this supplemental document, we provide:
\begin{itemize}
    \item Additional implementation details of \MethodName{},
    \item Experimental details of baseline methods,
    \item Additional evaluation details,
%    \item User study,
    % \item Additional quantitative comparison,
    \item Additional analysis,
    \item Additional comparison, and
    \item Additional visual results.
    
\end{itemize}

% \wj{Add OMSM multi modality?
% OMSM generates diverse object motions by using different Gaussian noise.
% }

\section{Additional Implementation Details of \MethodName{}}
\subsection{Network Architecture}
%\paragraph{Object Motion Synthesis Model}
The VAE encoders and decoders, and denoising U-Nets of the object motion synthesis model (OMSM) and of the flow-conditioned video synthesis model (FVSM) adopt the network architectures of Stable Video Diffusion~\cite{blattmann2023stable}.
For the flow encoder of FVSM, we adopt the CNN encoder from CameraCtrl~\cite{he2024cameractrl}, modifying it to process two-channel optical flow maps instead of six-channel Pl\"{u}cker embeddings.
The flow encoder produces multi-level flow embeddings $\{\zeta_{(t,l)}\}^{T,L}_{t=1,l=1}$ for the \textit{t}-th frame at level $l$, where $T=14$ and $L=4$.
To incorporate the optical flow condition into the denoising U-Net, the multi-level flow embeddings are added to the intermediate feature maps within the U-Net's encoder.
Each intermediate feature map matches the resolution and channel size of the corresponding flow embedding at the encoder's depth level $l$.

% \paragraph{Effectivenss of using the curated dataset}
% \wj{
% 추가할지 말지 고민.
% Comparison: OMSM w/ full data VS OMSM w/ curated data
% }

\subsection{Experimental Details}
% For training OMSM and FVSM, we use the AdamW optimizer \cite{loshchilov2017decoupled} with learning rate of 0.00003.
For training OMSM and FVSM, we use a learning rate of 0.00003 with the AdamW optimizer \cite{loshchilov2017decoupled}.
FVSM is trained over approximately two days using 16 A100 GPUs.
OMSM is trained on the entire dataset for about three days using 8 A100 GPUs, followed by fine-tuning on the curated dataset for an additional 1.5 days.
As explained in the main paper, we apply adaptive normalization for optical flow maps, following Li et al.~\cite{li2024generative}.
Specifically, we use different scale factors for the normalization of $x$- and $y$-directional optical flow vectors.
The scale factors of (18, 12) and (45, 24) are used to normalize flow-map data for OMSM and FVSM, respectively.

Following Stable Video Diffusion~\cite{blattmann2023stable}, we adopt the EDM framework~\cite{karras2022elucidating} for both training and inference, and apply linearly increasing classifier-free guidance during inference.
For training FVSM, we only modified the timestep sampling strategy of the EDM framework.
Inspired by T2I-Adapter~\cite{mou2024t2i}, we introduce a quadratic timestep sampling strategy to enable FVSM to more effectively leverage the input flow condition for structural content generation. 
Specifically, FVSM is trained primarily on highly noised data with large timesteps.

To achieve this, timesteps are uniformly sampled within the range [0, 1], squared, and subtracted from 1.
The resulting values are then scaled to match the range of (-3.66, 3.66), which roughly aligns with the timestep range used in the EDM framework.
This approach enables the denoising U-Net in FVSM to better learn structural content generation by leveraging the flow map condition, thereby enhancing its capability for effective camera control.

\subsection{Off-the-shelf Models Used in \MethodName{}}
We employ several off-the-shelf models in our framework: a single-image 3D estimation network~\cite{yang2024depth}, an optical flow estimation network~\cite{teed2020raft}, and a segmentation network~\cite{ravi2024sam} for moving object detection.

\paragraph{Single-image 3D estimation network.}
We use Depth Anything V2~\cite{yang2024depth} for the single-image 3D estimation network. Specifically, we use its fine-tuned version for metric depth estimation, which has a ViT-base encoder and is trained using the Hypersim dataset.

\paragraph{Optical flow estimation network.}
We use RAFT \cite{teed2020raft} for the optical flow estimation network.
Network outputs are iteratively updated 20 times to obtain the final optical flow map.

\paragraph{Moving object segmentation network.}
In the flow integration stage, we use a binary mask for moving objects.
To obtain the mask, we use an open-set segmentation method, Grounded-SAM 2, which integrates an open-set object detection model~\cite{liu2023grounding} and a foundation segmentation model~\cite{ravi2024sam}.
This method takes a text prompt and predicts masks indicating subjects related to the input text prompt.
To obtain masks for moving objects, we use "moving object." as the input text prompt.
We do not use the obtained mask if the number of pixels in the mask is more than 50\% of the total image pixels.

\paragraph{Temporally-consistent video editing.}
For temporally-consistent video editing using FloVD, we employ an off-the-shelf optical flow estimator and image editing tool.
We use RAFT~\cite{teed2020raft} and InfEdit~\cite{xu2023inversion} for the optical flow estimation and first frame editing, respectively.

% Our framework using FVSM enables temporally-consistent video editing at no extra cost.
% A video can be edited as follows.
% First, we obtain optical flow maps from the video by using an off-the-shelf optical flow estimator~\cite{teed2020raft}.
% We then edit the first frame of the input video using an off-the-shelf image editing tool, e.g., InfEdit~\cite{xu2023inversion}.
% We synthesize a video by using FVSM with the edited first frame and estimated optical flow maps as inputs.
% As shown in \cref{fig:video_editing}, this simple strategy using our framework can produce temporally-consistent video editing results, thanks to our optical-flow-based approach.

% \wj{
% Depth Anything V2 - Metric depth
% Grounded SAM2. text prompt: "moving object"
% RAFT - iteration 20
% }

\begin{table*}[!t]
\centering
\resizebox{\linewidth}{!}{
    \setlength\tabcolsep{1.5pt}
    \begin{tabular}{l|c|c|ccc|ccc|ccc|ccc}
    \toprule[1pt]
                    & Training & Timestep & \multicolumn{3}{c|}{Pexels-random} & \multicolumn{3}{c|}{Pexels-small ($<20$)} & \multicolumn{3}{c|}{Pexels-med. ($<40$)} & \multicolumn{3}{c}{Pexels-large ($\ge40$)}  \\
                    & Data & Strategy      & FVD ($\downarrow$)            & FID ($\downarrow$)        & IS ($\uparrow$)           & FVD ($\downarrow$)            & FID ($\downarrow$)        & IS ($\uparrow$)          & FVD ($\downarrow$)         & FID ($\downarrow$)        & IS ($\uparrow$)         & FVD ($\downarrow$)            & FID ($\downarrow$)        & IS ($\uparrow$)        \\ \hline
    Baseline    & RE10K & QTS  & 157.99   & 39.61  & 11.19 &  241.61  & \textbf{22.01}  & 11.09 & 334.06     & 22.30      & 11.17     & 363.04      & 23.17        & 12.05         \\
    \hspace{1mm} + OMSM & RE10K & QTS  & 104.92 & 36.33 & 11.51 & 231.35 & 22.43 & 11.44  & 206.38     & \textbf{20.53}     & 11.62      & 229.05       & \textbf{20.95} & 12.65   \\       
    \hspace{1mm} + large-scale data  & Internal & QTS  & \textbf{91.55}  & \textbf{35.66} & \textbf{11.63} & \textbf{220.65}   & 22.49       & \textbf{11.58}    & \textbf{183.14} & 20.71 & \textbf{11.68} & \textbf{207.39} & 21.12   & \textbf{12.95}    \\      \hline
    
    Baseline    & RE10K & EDM  & 148.42 & 39.92 & 11.23 &  238.85 & 22.16 & 11.07 & 309.28 & 22.05 & 11.28  & 335.02 & 22.91 & 12.15  \\
    \hspace{1mm} + OMSM & RE10K & EDM  & 95.31  & 36.90 & 11.43 & 217.24 & 22.13 & 11.44 & 186.21 & 20.12     & \textbf{11.81} & 201.27 & 20.45 & 12.71    \\       
    \hspace{1mm} + large-scale data  & Internal & EDM & \textbf{80.74}  & \textbf{35.65} & \textbf{11.73} & \textbf{212.03}   & \textbf{21.79} & \textbf{11.62} & \textbf{165.78} & \textbf{19.73} & 11.684 & \textbf{177.45} & \textbf{20.02}     & \textbf{12.88}    \\   
    \bottomrule[1pt]
    \end{tabular}
}
\vspace{-3mm}
\caption{
Comprehensive quantitative ablation study of our main components.
}
\vspace{-2mm}
\label{table:additional_ablation}
\end{table*}

% Baseline    & RE10K  & QTS & 157.99   & 39.61  & 11.19       \\
%     \hspace{1mm} + OMSM & RE10K  & QTS & 104.92 & 36.33 & 11.51   \\       
%     \hspace{1mm} + large-scale data  & Internal  & QTS & \textbf{91.55}  & \textbf{35.66} & \textbf{11.63}   \\  
%     \hline
%     Baseline    & RE10K & EDM & 148.42 & 39.92 & 11.23  \\
%     \hspace{1mm} + OMSM & RE10K & EDM & 95.31  & 36.90 & 11.43     \\       
%     \hspace{1mm} + large-scale data  & Internal & EDM & \textbf{80.74}  & \textbf{35.65} & \textbf{11.73} \\   
%     \bottomrule[1pt]
%     \end{tabular}

\begin{figure}[!t]
\centering
\begin{tabular}{@{}c}
\includegraphics[width=\columnwidth]{fig_supple/benchmark_example.pdf} \\
\end{tabular}
\vspace{-3mm}
\caption{
Visual examples of each benchmark dataset, categorized according to the degree of object motion.
}
\vspace{-3mm}
\label{fig:benchmark_example}
\end{figure}

\section{Experimental Details of Baseline Methods}
We compare our method against baseline methods for camera-controllable video synthesis~\cite{wang2024motionctrl, he2024cameractrl, guo2023animatediff, yang2024direct}.
Among these, MotionCtrl~\cite{wang2024motionctrl} and CameraCtrl~\cite{he2024cameractrl} support detailed camera control by utilizing camera parameters as input, whereas AnimateDiff~\cite{guo2023animatediff} and Direct-a-Video~\cite{yang2024direct} support basic camera control operations, such as translation and zoom.
For all the baseline methods, we used the official checkpoints and inference code provided in their respective GitHub repositories.

\paragraph{MotionCtrl}
We use the official PyTorch implementation of MotionCtrl~\cite{wang2024motionctrl}.
To ensure a fair comparison with our method, which is based on Stable Video Diffusion~\cite{blattmann2023stable}, we utilize the official variant of MotionCtrl that employs Stable Video Diffusion (\href{https://github.com/TencentARC/MotionCtrl}{https://github.com/TencentARC/MotionCtrl}).

\paragraph{CameraCtrl}
We use the official PyTorch implementation of CameraCtrl~\cite{he2024cameractrl}.
To ensure a fair comparison with our method, which is based on Stable Video Diffusion~\cite{blattmann2023stable}, we utilize the official variant of CameraCtrl that employs Stable Video Diffusion (\href{https://github.com/hehao13/CameraCtrl}{https://github.com/hehao13/CameraCtrl}).

\paragraph{AnimateDiff}
We use the official PyTorch implementation of AnimateDiff~\cite{guo2023animatediff}. The official codes can be found in (\href{https://github.com/guoyww/AnimateDiff}{https://github.com/guoyww/AnimateDiff}).
To control pre-defined camera trajectories, such as zoom and pan, AnimateDiff provides fine-tuned models tailored for each camera trajectory.
Thus, we utilize these fine-tuned models for camera control during video generation.
Additionally, we use the model from Realistic Vision as a backbone for AnimateDiff, as it is most closely aligned with generating natural images.

\paragraph{Direct-a-Video}
We use the official PyTorch implementation of Direct-a-Video~\cite{yang2024direct}.
The official codes can be found in (\href{https://github.com/ysy31415/direct_a_video}{https://github.com/ysy31415/direct\_a\_video}).
Direct-a-Video controls basic camera motions using camera parameters such as $x$-pan ratio, $y$-pan ratio, and zoom ratio.
For our experiments, we set the pan ratio to 0.3 and used scales of 0.8 and 1.2 for zoom-in and zoom-out ratios, respectively.
% (\href{https://github.com/ysy31415/direct_a_video}{https://github.com/ysy31415/direct\_a\_video})

\begin{table}[!t]
\centering
\resizebox{\columnwidth}{!}{
    \begin{tabular}{l|ccc}
    \toprule[1pt]
                    & mRotErr ($^\circ$) & mTransErr        & mCamMC     \\ \hline
    Ours w/ EDM     & 1.70               & 0.0983           & 0.1010    \\
    Ours w/ QTS   & 1.43               & 0.0869           & 0.0887    \\
         
    \bottomrule[1pt]
    \end{tabular}
}
\vspace{-3mm}
\caption{
Analysis of employing different timestep sampling strategies for camera controllability.
}
\vspace{-4mm}
\label{table:timestep_strategy}
\end{table}

\begin{figure*}[!t]
\centering
\begin{tabular}{@{}c}
\includegraphics[width=\linewidth]{fig_supple/limitation.pdf} \\
\end{tabular}
\vspace{-3mm}
\caption{
A visual example of the limitation of FloVD.
}
% \vspace{-3mm}
\label{fig:limitation}
\end{figure*}

\section{Additional Details for Evaluation Protocol}
\subsection{Camera Controllability}
To obtain each video clip in the evaluation dataset, we first select a middle frame within the whole video frames as the first frame, and then choose 13 additional frames at intervals of four frames starting from the first frame, resulting in a total of 14 frames.
Then, we obtain camera parameters corresponding to these selected frames to serve as the ground-truth camera parameters for the evaluation set.
For the camera parameters estimated from synthesized videos, we normalize the translation vectors using a scale factor to account for scene-specific scale variations, following CamI2V~\cite{zheng2024cami2v}.
Specifically, the translation vectors are divided by a scene-specific scale factor.
This scale factor is determined based on the $\mathcal{L}_2$ distance between the locations of the first camera and the farthest camera in the scene.

% Corresponding camera parameters are extracted for these selected frames to serve as the ground-truth camera parameters for the evaluation set.

% other 13 frames every four frames from the first frame, obtaining 14 frames in total.
% We then obtain camera parameters corresponding to the selected frames for the ground-truth camera parameters of the evaluation set.
% After camera parameters are estimated from synthesized videos, the translation vectors are divided by a scale factor for scale normalization of each scene, following CamI2V~\cite{zheng2024cami2v}.
% The scale factor is determined using the $\mathcal{L}_2$ distance between the location of the first and farthest cameras.

\subsection{Video Synthesis Quality}
% \wj{[추가] 어떤 기준으로 camera motion 없는 것들 모았는지? background optical flow 기준 등.}
As explained in the main paper, we provide three benchmark datasets of real-world videos categorized by small, medium, and large object motions to evaluate the object motion synthesis quality.
To obtain videos with minimal camera motions, we first obtain optical flow maps from the Pexels dataset~\cite{pexels_dataset}, and then filter out videos whose average magnitude of the optical flow vectors of the background is larger than 1.0.
\cref{fig:benchmark_example} shows several visual examples from each benchmark dataset.
The first set primarily features landscapes or objects with minimal motions, while the third set typically consists of objects with notable motions.

\section{Additional Analysis}
In the following, we provide additional analysis of our method in terms of comprehensive ablation study, timestep sampling strategy, scaling effect, and training FVSM using camera parameters.

% \section{Additional Quantitative Ablation Study}
\subsection{Additional Quantitative Ablation Study}
\cref{table:additional_ablation} reports the comprehensive evaluation of our main components using the whole benchmark datasets for video synthesis quality.
Introducing each component mostly enhances evaluation metrics, in both cases using the quadratic timestep sampling strategy (QTS) or EDM framework~\cite{karras2022elucidating}.

\subsection{Timestep Sampling Strategy}
As stated in Sec.~5.1 of the main paper, we adopt the quadratic timestep sampling strategy (QTS) for better camera controllability, instead of the timestep sampling strategy of the EDM framework~\cite{karras2022elucidating} used in Stable Video Diffusion~\cite{blattmann2023stable}.
Our model using QTS shows slightly compromised video synthesis quality compared to our model using EDM~(\cref{table:additional_ablation}).
Nevertheless, our model with QTS still demonstrates better performance than the previous methods~(Tab.~2 in the main paper).
% (\cref{table:sample_quality}).
Moreover, QTS enhances the camera controllability of FVSM~(\cref{table:timestep_strategy}).
This improved camera controllability results from increased chances of training with highly noised data, allowing our model to effectively leverage flow conditions for structural content generation.

\begin{table}[!t]
\centering
\resizebox{\columnwidth}{!}{
    \begin{tabular}{l|cc|c}
    \toprule[1pt]
    $\#$ of Data         & 70K       & 300K      & 500K (Original)     \\ \hline
    FVD ($\downarrow$)   & 191.73    & 188.22    & 177.45    \\
    \bottomrule[1pt]
    \end{tabular}
}
\vspace{-3mm}
\caption{
Analysis of the scaling effect using the Pexels-large benchmark dataset and the FVD scores.
}
\vspace{-4mm}
\label{table:scaling_effect}
\end{table}

\subsection{Scaling effect}
By utilizing optical flow during training instead of camera parameters, our method can leverage arbitrary training datasets, allowing for the use of an arbitrary number of training datasets.
Thus, we investigate whether increasing the size of the training dataset could enhance the performance of our approach.

To assess this, we constructed two subsets randomly sampled from our full internal dataset, containing 70K and 300K pairs of video frames with corresponding optical flow maps, respectively. 
Notably, the RealEstate10K dataset~\cite{zhou2018stereo} includes around 70K videos, fewer compared to the 500K pairs available in our full internal dataset.
We trained two variant models of FVSM using these subsets. 
As illustrated in \cref{table:scaling_effect}, the performance of our method on the Pexels-large benchmark dataset consistently improves as the training dataset size increases, indicating the potential for further performance gains with even larger datasets. Additionally, we anticipate that adopting transformer-based architectures could further enhance performance with larger datasets.

\begin{table}[!t]
\centering
\resizebox{\columnwidth}{!}{
    \begin{tabular}{l|ccc}
    \toprule[1pt]
                         & mRotErr ($^\circ$) & mTransErr        & mCamMC     \\ \hline
    Ours w/ CamParams    & 1.76               & 0.1016           & 0.1039    \\
    Ours w/ Flow (final) & 1.43               & 0.0869           & 0.0887    \\
         
    \bottomrule[1pt]
    \end{tabular}
}
\vspace{-3mm}
\caption{
Analysis of training FVSM using camera parameters.
}
\vspace{-2mm}
\label{table:fvsm_camparam}
\end{table}

\subsection{Training FVSM using Camera Parameters}
Our proposed training strategy employs optical flow maps rather than camera parameters to eliminate the dataset restriction.
Although we may use camera parameters for training when available in the dataset, we found that this does not improve the performance.
To show this, we train FVSM using camera flow maps derived from estimated depth and camera parameters, rather than optical flow estimated from the video dataset.
As shown in~\cref{table:fvsm_camparam}, the results show degraded performance compared to the original one.
This performance degradation came from depth estimation errors, as we utilize the off-the-shelf single-image 3D estimation network~\cite{yang2024depth}.

\subsection{Visual Example on Limitation}
Despite using FVSM trained on the large-scale dataset, errors derived from both the object motion synthesis model and the moving object segmentation model can produce unnatural object motions.
\cref{fig:limitation} shows a visual example on the limitation, particularly in the ring pull of the can (red arrow).

% We evaluate the quality of synthesized video frames using the Frechet Inception Distance (FID)~\cite{heusel2017gans}, as presented in~\cref{table:quan_comp_supple}.
% For the benchmark datasets with medium and large object motions, our method achieves superior FID scores over previous approaches, MotionCtrl~\cite{wang2024motionctrl} and CameraCtrl~\cite{he2024cameractrl}.
% Notably, MotionCtrl exhibits degraded FID scores due to artifacts in synthesized video frames, as shown in Fig.~6 of the main paper and~\cref{fig:cam_control_supple2}.

% average FVD
% FID
% KID?
% FVD per camera trajectory

\begin{table}[!t]
\centering
\resizebox{\columnwidth}{!}{
    \begin{tabular}{l|ccc}
    \toprule[1pt]
                & Pexels-small       & Pexels-med.      & Pexels-large     \\ \hline
    MotionCtrl  & 0.884               & 0.881           & 0.875    \\
    CameraCtrl  & 0.913               & 0.913           & 0.910    \\
    Ours        & \textbf{0.917}      & \textbf{0.916}  & \textbf{0.911}    \\
    \bottomrule[1pt]
    \end{tabular}
}
\vspace{-3mm}
\caption{
Quantitative comparison on visual consistency using CLIP-Similarity.
}
\vspace{-3mm}
\label{table:clip_similarity}
\end{table}

\begin{figure*}[!t]
\centering
\begin{tabular}{@{}c}
\includegraphics[width=\linewidth]{fig_supple/cam_control_challenge.pdf} \\
\end{tabular}
\vspace{-3.5mm}
\caption{
Limited scope of circular camera trajectory.
}
\vspace{-2mm}
\label{fig:cam_control_challenge}
\end{figure*}

\section{Additional Comparison}
In the following, we provide additional comparison against previous methods~\cite{wang2024motionctrl,he2024cameractrl} in terms of visual consistency, 3D scene consistency, and challenging camera motion.

\subsection{Visual Consistency}
To evaluate image-to-video fidelity, we measure CLIP-Similarity~\cite{radford2021learning} between synthesized videos and an input image.
\cref{table:clip_similarity} shows quantitative comparison results.
MotionCtrl~\cite{wang2024motionctrl} less effectively preserves visual consistency with input image due to visual artifacts, achieving the lowest scores, while ours achieves slightly higher scores than CameraCtrl~\cite{he2024cameractrl}.

\subsection{3D Scene Consistency}
Thanks to our 3D-based approach for camera-controllable video generation, FloVD can also provide 3D consistent video synthesis results.
To validate this, we evaluate 3D scene consistency by employing a NeRF-based approach~\cite{mildenhall2021nerf}. Specifically, we first generate video frames with a forward-facing, circular camera trajectory. We then split these synthesized frames into training and test sets, and reconstruct NeRF using the training set. 
Lastly, we compute PSNR by comparing the test-set frames against the corresponding images rendered from NeRF.

\cref{fig:NeRF_Comparison} shows rendered frames at test-set viewpoints from the reconstructed NeRF.
FloVD shows high-quality rendered images compared to those of the previous methods~\cite{wang2024motionctrl,he2024cameractrl}, demonstrating more 3D-consistent video synthesis results of our method.
\cref{table:3d_consistency} shows quantitative comparison on 3D scene consistency using the PSNR scores.
These results also demonstrate that our method achieves comparable or superior 3D scene consistency compared to others.

\begin{figure}[!t]
\centering
\begin{tabular}{@{}c}
\includegraphics[width=\linewidth]{fig_supple/NeRF_Comparison.pdf} \\
\end{tabular}
\vspace{-3mm}
\caption{
Qualitative comparison on 3D scene consistency using NeRF~\cite{mildenhall2021nerf} reconstruction.
}
\vspace{-2mm}
\label{fig:NeRF_Comparison}
\end{figure}

\begin{table}[!t]
\centering
\resizebox{0.9\columnwidth}{!}{
    \begin{tabular}{l|ccc}
    \toprule[1pt]
                & Horns               & Fern            & Trex     \\ \hline
    MotionCtrl  & 15.56               & 17.87           & 18.12    \\
    CameraCtrl  & 19.84               & \textbf{21.42}  & 20.71    \\
    Ours        & \textbf{21.55}      & 20.93           & \textbf{20.02}    \\
    \bottomrule[1pt]
    \end{tabular}
}
\vspace{-3mm}
\caption{
Quantitative comparison on 3D scene consistency using the PSNR scores.
}
\vspace{-4mm}
\label{table:3d_consistency}
\end{table}

\subsection{Challenging Camera Motion}
We provide a qualitative comparison of video synthesis capability for extreme camera motions.
Extreme camera poses (e.g., circular camera rotations) are still challenging in camera-controlled video synthesis, and all existing methods struggle with this issue. 
Nonetheless, our approach demonstrates higher robustness to extreme camera poses than others, due to our 3D-structure-based camera flow map.
\cref{fig:cam_control_challenge} shows that MotionCtrl~\cite{wang2024motionctrl} completely fails to follow the input camera parameters. In contrast, both CameraCtrl~\cite{he2024cameractrl} and our method generate results that reflect input camera parameters up to $72^\circ$. 
While both methods generate distorted images at $72^\circ$, our results exhibit fewer distortions.

\section{Additional Visual Results}
In this section, we provide additional visual results.
First, we qualitatively compare our method with AnimateDiff~\cite{guo2023animatediff} and Direct-a-Video~\cite{yang2024direct} using basic camera trajectories such as zoom and translation, as these methods are limited to those basic camera movements.
Next, we qualitatively compare our method with MotionCtrl~\cite{wang2024motionctrl} and CameraCtrl~\cite{he2024cameractrl}, which support more detailed camera control during video generation.
Lastly, we provide additional visual examples of the applications regarding temporally-consistent video editing and cinematic camera control.

\begin{figure*}[!t]
\centering
\begin{tabular}{@{}c}
\includegraphics[width=\linewidth]{fig_supple/application_dolly_zoom_sup.pdf} \\
\end{tabular}
\vspace{-3.5mm}
\caption{
Additional visual example of the dolly-zoom effect.
}
\vspace{-2mm}
\label{fig:dolly_zoom_sup}
\end{figure*}

\begin{figure}[!t]
\centering
\includegraphics[width=\linewidth]{fig_supple/application_video_editing_sup.pdf} \\
\vspace{-2.5mm}
\caption{
Additional visual example of the temporally-consistent video editing.
}
\vspace{-2mm}
\label{fig:video_editing_sup}
\end{figure}

\subsection{Using Basic Camera Trajectory}
\cref{fig:cam_control_supple4} presents a visual comparison using basic camera trajectories such as zoom-in and translation to left and right.
Unlike our method, which uses a single image as input, Direct-a-Video~\cite{yang2024direct} and AnimateDiff~\cite{guo2023animatediff} require text prompts as input.
Thus, we use text prompts of videos from the Pexels dataset~\cite{pexels_dataset} as input for these methods, while the first frame of the same video serves as input for our method.
As shown in~\cref{fig:cam_control_supple4}, our method synthesizes high-quality video frames with accurate camera control, while previous methods produce video frames with quality degradation.

% \wj{카메라 컨트롤 수행 시 엄밀하게 translation하지 않고 휘는 문제가 보이긴 함. 하지만, 이전 방법이 논문에서 pan을 한다고 주장하기 때문에 이를 지적하기 애매함. (실제로 direct-a-video는 translation을 학습시켰습니다..)}
% with inaccurate camera control.
% In particular, AnimateDiff synthesizes videos 

\subsection{Using Detailed Camera Trajectory}
\cref{fig:cam_control_supple1} and \cref{fig:cam_control_supple1_2} provide a visual comparison of synthesized video frames with detailed camera trajectory.
MotionCtrl~\cite{wang2024motionctrl} often fails to accurately follow the input camera trajectory, whereas both CameraCtrl~\cite{he2024cameractrl} and our method demonstrate accurate camera control performance.

\cref{fig:cam_control_supple2} provides additional visual comparison across all the methods.
Our method generates realistic object motion in the synthesized video frames, while previous methods often produce unnatural videos with artifacts.
In particular, CameraCtrl~\cite{he2024cameractrl} often synthesizes video frames without object motion, and MotionCtrl~\cite{wang2024motionctrl} often produces inconsistent foreground and background, as shown in~\cref{fig:cam_control_supple2}.
Additional visual examples can be found in~\cref{fig:cam_control_supple3}.
% \cref{fig:cam_control_supple3} provides additional visual examples of all the approaches for further comparison.

% Our method shows realistic object motion in synthesized video frames, while previous methods produce artifacts.
% Especially, CameraCtrl often synthesizes video frames without object motion, as shown in the first example of \cref{fig:cam_control_supple2}.
% \cref{fig:cam_control_supple3} further presents visual examples of all the approaches.

% \section{Details on 3D-aware optical flow acquisition}
% 물체와 카메라가 3차원에서 동시에 움직일 때,
% 3D-aware optical flow는 src view의 pixel coordinate가 target view pixel coordinate로 변환되는 과정을 통해 구할 수 있다.
% 먼저, depth와 camera intrinsics를 사용해 3D point cloud를 구한다.
% 이후, 3D point cloud는 object motion을 모사한 $T^o$를 통해 다른 3차원 좌표로 translation 되는데, 이때 $T^{3D,o}$는 non-homogeneous translation이며 정확한 함수를 알기 어렵다.
% 이후, 변환된 3차원 point cloud는 extrinsics를 사용해 target view 좌표계로 transformation 된다.
% 이후 카메라 모션으로 인해 변환된 3차원 point cloud를 target view image plane으로 projection하여 target view에서의 카메라 변환 pixel coordinates를 구할 수 있다.
% 이 coordinate에서 처음 coordinate를 빼면 camera motion flow를 구할 수 있다.
% 또한, $T^{3D,o}$를 target view로 projection하면 object motion flow를 구할 수 있다.
% 이때, motion flow, 즉 displacement를 camera parameter를 사용해 다시 warping함으로써 카메라 모션이 고려된 object motion flow를 구할 수 있다.
% displacement의 warping은 물체가 카메라와 수직한 평며 상에서 움직인다는 가정 하에 이루어지며, 실험적으로 에러가 크지 않음을 확인했다.
% 마지막으로, 이렇게 구해진 camera object motion flow를 더함으로써 최종적인 3D-aware optical flow를 구한다.

\subsection{Application}
In Sec.~5.5 of the main paper, we provide two applications using our framework: temporally-consistent video editing and cinematic camera control.
We provide additional visual examples of these applications.
\cref{fig:dolly_zoom_sup} and \cref{fig:dolly_zoom_sup} show additional examples of the dolly-zoom effect and temporally-consistent video editing result, respectively.

% \begin{equation}
% \vspace{-2mm}
% \begin{aligned}
% x_{t} &\sim K_{t}T^{c}_{s \xrightarrow{} t} T^{o}_{s \xrightarrow{} t} K^{-1}_{s} x_{s} d_{s} \\
%       &= K_{t}T^{c}_{s \xrightarrow{} t}(p + T^{3D,o}_{s \xrightarrow{} t}(p)) ~ (p=K^{-1}_{s} x_{s} d_{s}) \\
%       &= K_{t}T^{c}_{s \xrightarrow{} t}p + K_{t}T^{c}_{s \xrightarrow{} t}T^{3D,o}_{s \xrightarrow{} t}(p) \\
%       &=(x_{s}+f^{c}_{t}) + K_{t}T^{c}_{s \xrightarrow{} t}K^{-1}_{t}K_{t}T^{3D,o}_{s \xrightarrow{} t}(p) ~(f^{o}_{t}=K_{t}T^{3D,o}_{s \xrightarrow{} t}(p)) \\
%       &=(x_{s}+f^{c}_{t}) + \mathcal{W}_{s \xrightarrow{} t}(d_{s}, f^{o}_{t}), \\
% f_{t}&=x_{t}-x_{s}, \\
% f_{t}&=f^{c}_{t}+\mathcal{W}_{s \xrightarrow{} t}(d_{s}, f^{o}_{t}).
% \end{aligned}
% \end{equation}

\begin{figure*}[!t]
\centering
\includegraphics[width=\linewidth]{fig_supple/cam_control_supple_detailed1.pdf} \\
% \vspace{-3mm}
\caption{
Additional qualitative comparison of our method against MotionCtrl~\cite{wang2024motionctrl} and CameraCtrl~\cite{he2024cameractrl} using detailed camera trajectories.
MotionCtrl often fails to follow the input camera parameters during video generation.
}
% \vspace{-2mm}
\label{fig:cam_control_supple1}
\end{figure*}

\begin{figure*}[!t]
\centering
\includegraphics[width=\linewidth]{fig_supple/cam_control_supple_simple.pdf} \\
\vspace{-3mm}
\caption{
Additional qualitative comparison of our method against Direct-a-video~\cite{yang2024direct} and AnimateDiff~\cite{guo2023animatediff} using basic camera trajectories.
}
\vspace{-2mm}
\label{fig:cam_control_supple4}
\end{figure*}

\begin{figure*}[!t]
\centering
\begin{tabular}{@{}c}
\includegraphics[width=\linewidth]{fig_supple/cam_control_supple_detailed1_2.pdf} \\
\end{tabular}
% \vspace{-3mm}
\caption{
Additional qualitative comparison of our method against MotionCtrl~\cite{wang2024motionctrl} and CameraCtrl~\cite{he2024cameractrl} using detailed camera trajectories.
MotionCtrl often fails to follow the input camera parameters during video generation.
}
% \vspace{-2mm}
\label{fig:cam_control_supple1_2}
\end{figure*}

\begin{figure*}[!t]
\centering
\begin{tabular}{@{}c}
\includegraphics[width=\linewidth]{fig_supple/cam_control_supple_detailed2.pdf} \\
\end{tabular}
\vspace{-3mm}
\caption{
Additional qualitative comparison of our method against MotionCtrl~\cite{wang2024motionctrl} and CameraCtrl~\cite{he2024cameractrl} using detailed camera trajectories.
Our method produces more natural object motion, while CameraCtrl produces a foreground object without motions, and MotionCtrl produces artifacts.
}
\vspace{-2mm}
\label{fig:cam_control_supple2}
\end{figure*}

\begin{figure*}[!t]
\centering
\begin{tabular}{@{}c}
\includegraphics[width=\linewidth]{fig_supple/cam_control_supple_detailed3.pdf} \\
\end{tabular}
\vspace{-3mm}
\caption{
Additional qualitative comparison of our method against MotionCtrl~\cite{wang2024motionctrl} and CameraCtrl~\cite{he2024cameractrl} using detailed camera trajectories.
}
\vspace{-2mm}
\label{fig:cam_control_supple3}
\end{figure*}
